# Supplementary material for: Analyzing Transformers in Embedding Space
Source: arXiv:2209.02535 source file (2023-12-24)
Supplement: Supplementary file 1 [file 11_appendix_summary.tex]

%\appendix

\pagebreak
\section{Executive Summary}
\label{appendix:exec_sum}
 \textit{Important note}: In PyTorch, the kernel of \verb|nn.Linear| is \textit{transposed} (i.e., it implements the function $\textrm{Linear}(x) = x W^T + b$). Thus, we expect to get the $W^T$ as the weight matrix.  

% \begin{figure*}
\begin{lstlisting}[language=Python]
# L = current layer
# H = number of heads
# d = hidden dimension

# attention projection matrices
W_Q_heads[L] = W_Q[L].reshape(d, H, d // H).transpose(0, 1) # (H, d, d // H)
W_K_heads[L] = W_K[L].reshape(d, H, d // H).transpose(0, 1) # (H, d, d // H)
W_V_heads[L] = W_V[L].reshape(d, H, d // H).transpose(0, 1) # (H, d, d // H)

W_O_heads[L] = W_O[L].reshape(H, d // H, d)  # (H, d // H, d)

# interaction matrices
W_QK[L] = W_Q_heads[L] @ W_K_heads[L].transpose(-1, -2) # (H, d, d)
W_VO[L] = W_V_heads[L] @ W_O_heads[L]                   # (H, d, d)

# weights interpretations
K_emb[L] = K[L] @ E2.T
V_emb[L] = V[L] @ E1
W_QK_emb[L] = E2 @ W_QK[L] @ E2.T
W_VO_emb[L] = E2 @ W_QK[L] @ E1
\end{lstlisting}
% \caption{PyTorch code for computing projected parameters}
% \end{figure*}
Further vectorization can be applied here if all layer weights are concatenated along a new axis.
\par In equations: 

\begin{center}
\begin{tabular}{ c | c c c }
   & \textbf{Symbol} & \textbf{Projection} & \textbf{Approx. Projection} \\
 FF values & $v$ & $vE_1$ & $v E$ \\ 
 FF keys & $k$ & $kE_2^\top$ & $kE$ \\
 Att. Query-Key  & $\WQK^i$ & $E_2 \WQK^i E_2^\top$ & $E^\top \WQK^i E$ \\  
 Att. Value-Output  & $\WVO^i$ & $E_2 \WVO^i E_1$ & $E^\top \WVO^i E$ 
\end{tabular}
\end{center}
